# Supplementary material for: Few-Shot Anaphora Resolution in Scientific Protocols via Mixtures of In-Context Experts
Source: arXiv:2210.03690 source file (2022-11-14)
Supplement: Supplementary file 1 [file appendix.tex]

\subsection{Dataset construction details} 

\Max{We can show difference between our annotations and other datasets, similar to Zhou and Choi (2018)}

\paragraph{Anaphor Selection} 
- they (What is the scientific term for this-- pronominal expressions?)
- The mixture 

\paragraph{Atomic Antecedents} 
- Define: not his, not her, but names/ingredients
- Practically, select the first appearing terms in a coreference clusters

\paragraph{Terminology and Notation} Most previous work on few-shot learning and in-context learning work on tasks where an example is often defined at the sentence-level. As such, the number of shot $k$ often means $k$ sentences. For document-level tasks such as coreference and anaphora resolution, this definition becomes slightly more complicated, as $k$ is no longer the number of sentences. Should we then define $k$ to be the fine-grained number of examples (i.e. anaphor-set-of-antecedents pairs), or a more coarse-grained number of documents?

- Another reason why it's not as simple, is the consideration of baselines that was used. 

- "Document-level" few-shot learning
- Document and examples 
- What k means 
- How we control the variance 

\Max{Some concerns: (1) I'm a little anxious on defining the task like this. Are there any previous work that support this definition?
(2) Should we restrict $|m|$ > 1 i.e. only consider anaphors with multiple antecedents?
TODO: Modify with the new definition of $k$, according to discussion with Fan}

\begin{table*}[!h]
\centering
\scalebox{1.0}{
\begin{tabular}{lcccccccccccccccc}
\toprule
\textbf{Datasets} & \multicolumn{6}{c}{\textbf{CheEMU-Ref}} & \multicolumn{6}{c}{\textbf{RecipeRef}} & \multicolumn{4}{c}{\textbf{ARRAU}}\\
\cmidrule(l{5pt}r{5pt}){2-7} \cmidrule(l{5pt}r{5pt}){8-13} \cmidrule(l{5pt}r{5pt}){14-17} 
 $k$-shot & \textit{4} & \textit{8} & \textit{16} & \textit{32} & \textit{64} & \textit{full} & \textit{4} & \textit{8} & \textit{16} & \textit{32} & \textit{64} & \textit{full} & \textit{4} & \textit{8} & \textit{16} & \textit{full} \\
\hline
\textsc{Recent-5} & & & & &\\
\textsc{Recent-all} & & & & &\\
\textsc{Random} & & & & &\\
\textsc{Fang et al. 2021} & & & &  & &\\
Yu et al. 2021 & & & &  & &\\
\hline
GPT2-XL & 18.9 &  & &\\
T5-3B & 45.7 &&  & &\\
T0-3B & 40.1 & &  & &\\
\hline 
\textsc{SingleRandom} & & & & & &\\
\textsc{SingleSimilar} & & & & &\\
\textsc{EnsembleRandom} & & & & &\\
\textsc{EnsembleSimilar} & & & & &\\
\bottomrule
\end{tabular}
}
\caption{Our main results on the test sets (subset for ChEMU-Ref and RecipeRef; full for ARRAU) using GPT-J as foundation model. The first row indicates the result by training the TODO baseline on the full train set. For the rest, we report the results using $k=16$ examples in $\mathcal{D}_{train}$ (full results on different $k$ in the Appendix TODO). We report the mean and standard deviation across 3/5 different $\mathcal{D}_{train}$ splits (TODO reference section). \Max{TODO: Where to put fully-supervised?}}
\label{tab:main}
\end{table*}

\subsection{Full experiments results}
\begin{table*}[!h]
\centering
\scalebox{1.0}{
\begin{tabular}{lccccccccc}
\toprule
\multirow{2}{*}{\textbf{Datasets}} & \multicolumn{3}{c}{\textbf{CheEMU-Ref}} & \multicolumn{3}{c}{\textbf{RecipeRef}} & \multicolumn{3}{c}{\textbf{ARRAU}}\\
\cmidrule(l{5pt}r{5pt}){2-4} \cmidrule(l{5pt}r{5pt}){5-7} \cmidrule(l{5pt}r{5pt}){8-10} 
 & Avg_{(Std)} & Best & Worst & Avg_{(Std)} & Best & Worst & Avg_{(Std)} & Best & Worst \\
\hline
\textsc{Recent-5} & 45.7 & & & &\\
\textsc{Recent-all} & 44.0 & & & &\\
\textsc{Random} & 27.8 & & & &\\
\textsc{Fang et al. 2021} & & & &  & &\\
Yu et al. 2021 & & & &  & &\\
\hline
Extractive QA & & & &  & &\\
GPT2-XL & 18.9 &&  & &\\
T5-3B & 45.7 &&  & &\\
T0-3B & 40.1 & &  & &\\
\hline 
\textsc{SingleRandom} & & & & & &\\
\textsc{SingleMostSimilar} & & & & &\\
\textsc{EnsembleRandom} & 63.3 & & & &\\
\textsc{EnsembleSimilar} & 63.8 & & & &\\
\bottomrule
\end{tabular}
}
\caption{Best+Worse+Average Case performance, for k=32}
\label{tab:detailed}
\end{table*}

\subsection{Terminology and Notation}
\begin{table*}[!t]
\centering
\begin{tabular}{ll}
\hline
Notation & Description\\
\hline
$X$ & An example for our task, $X = (D, a)$ \\
$D$ & Input document \\
$a$ & Input anaphor \\
$E$ & Set of gold antecedents $E = \{e_1, ..., e_m\}$. E for entity \\
$\hat{E}$ & Predicted antecedents $\hat{E} = \{\hat{e}_1, ..., \hat{e}_{m'}\}$ \\
$k$ & Number of examples ("shot") in $D_{train}$\\
$n_C$ & Number of in-context examples \\
$D_{train}$ & Training data. Assumed to be small (e.g. $|D_{train}| < 100)$\\
$\mathcal{D}_{dev}$ & Development data. Assumed to be $|\mathcal{D}_{dev}| \leq |\mathcal{D}_{train}|)$\\
$\mathcal{D}_{test}$ & Test data\\
$\mathcal{T}$ & Template function that converts input into LM-ready text \\
$\mathcal{T}(X)$ & template-based text without gold antecedents \\
$\mathcal{T}(X, E)$ & template-based text with gold antecedents \\
$\mathbcal{N}_{X_{test}}$ & Set of top-$t$ similar examples to $X_{test}$ \\
$\mathcal{C}$ & Set of in-context configurations/permutations \\
$C$ & A single in-context configuration \\
$y_{\hat{E}}$ & Output of the language model and linearization of predicted antecedents \\
\hline
\end{tabular}
\caption{Notation table}
\label{TODO}
\end{table*}

\begin{table*}[!t]
\centering
\begin{tabular}{ll}
\hline
Terminology & Description\\
\hline
template & \\
prompt & input into LM\\ 
generated text & output of LM\\ 
context & \\ 
in-context examples & \\
in-context configuration & converted template of all the in-context examples, \\ 
& minus the template of test example \\
\hline
\end{tabular}
\caption{Terminology table}
\label{TODO}
\end{table*}

\subsection{Hyperparameter tuning experiments}
- On dev set 
- Hyperparameters: t (in top-t), p_m_pre, p_m_post

\paragraph{Different prompt templates}
\label{sec:prompt_format}
This experiment studies how different prompt templates effect performance. This can be interesting, depending on the type of the answers (eg "who" vs "what"), but in general I expect the results does not change much across templates (assume we experiment with reasonable templates). Assume we have 4-5 reasonable templates. Experimental Dataset: On dev set (sub-sample: how much data is reasonable?); dataset: ChemuRef/ARRAU. Reference tables: Table 3/4 of Lu et al 2022. Fill in results of \ref{tab:prompt_template}.
\begin{table}[!t]
\centering
\begin{tabular}{lccccc}
\hline
 & T1 & T2 & T3 & T4 & T5\\
\hline
SingleRandom & & & & &\\
SingleMostSimilar & & & & &\\ 
SingleOracle & & & & &\\
EnsembleRandom & & & & &\\
EnsembleSimilar & & & & &\\
EnsembleOracle & & & & &\\
\hline
\end{tabular}
\caption{Results on how different templates (T1-T5) affect the performance of different in-context models. We report the mean and standard deviation across 5 different splits of $k=16$ \Max{This can also be in graph format to show the variance reduction for ensemble vs. single across different prompts}}
\label{tab:prompt_template}
\end{table}

\paragraph{In-context ordering}
This experiment measures the effect of different in-context ordering in our problem setting. The question: given a single test example $X_{test}$, $\mathcal{D}_{train}$ of size $k=16$,  and 100 different prompts to ensemble, what are the possible orderings of these prompts? Assume each prompt contains 2 in-context examples (assumption across this project). A few methods to consider: 
\begin{itemize}
    \item MostSimilar: for prompt, we order the examples most similar closest to $X_{test}$. Since ordering matters, we need between 14-15 examples. Using all 16 gives us $16\times15/2 = 120$ prompts.
    \item LeastSimilar: reverse of MostSimilar
    \item Mixed: Top-10 + BruteForce all pairs. Current approach, generate 100 prompts 
\end{itemize}
The evaluation dataset is ChemuRef dev set (TODO \# of examples). Results filled in Table \ref{tab:in_context_ordering}. I actually don't know what the expectation will be for this.
\begin{table}[!t]
\centering
\begin{tabular}{lcccc}
\hline
 & P & R & F1 & Acc \\
\hline
MostSimilar & & & & \\
LeastSimilar & & & & \\
Mixed & & & & \\
\hline
\end{tabular}
\caption{The effects of different prompt ordering on the performance, using $\mathcal{D}_{train}$ of size $k=16$}
\label{tab:in_context_ordering}
\end{table}

\paragraph{In-context example retrieval}
This is to see if top-t similarity + brute force has any advantage; or whether it's the ensembling that does the heavy lifting of reducing variance. The question: given a single test example $X_{test}$, $\mathcal{D}_{train}$ of size $k=16$,  and 100 different prompts to ensemble, how do we choose these prompts? A few methods:
\begin{itemize}
    \item Random: randomly sample 100 prompts, out out $k^2 = 16^2 = 256$ possible prompts.
    \item Top-10 + BruteForce all pairs. Current approach, generate 100 prompts. The variance is then in the retrieval module. We experiment with BM25, ProcBERT, SentenceRoberta, SentenceT5
\end{itemize}
The evaluation dataset is ChemuRef dev set (TODO \# of examples). Results filled in Table \ref{tab:in_context_retrieval}.

\begin{table}[!t]
\centering
\begin{tabular}{lcccc}
\hline
 & P & R & F1 & Acc \\
\hline
Random & & & & \\
BM25 & & & & \\
ProcBERT & & & & \\
SentenceRoBERTa & & & & \\
SentenceT5 & & & & \\
\hline
\end{tabular}
\caption{Different in-context retrieval methods, using $\mathcal{D}_{train}$ of size $k=16$}
\label{tab:in_context_retrieval}
\end{table}

\paragraph{Numbers of In-context Examples}
Varying from 0-2 (max\_context\_len would allow at most 2 anyway). This is mostly to convince on using 2 in-context examples. We can move this to Appendix. Results will be similar to Figure \ref{fig:num_in_context_examples} 

\begin{figure}[!t]
    \centering
    \includegraphics[scale=0.50]{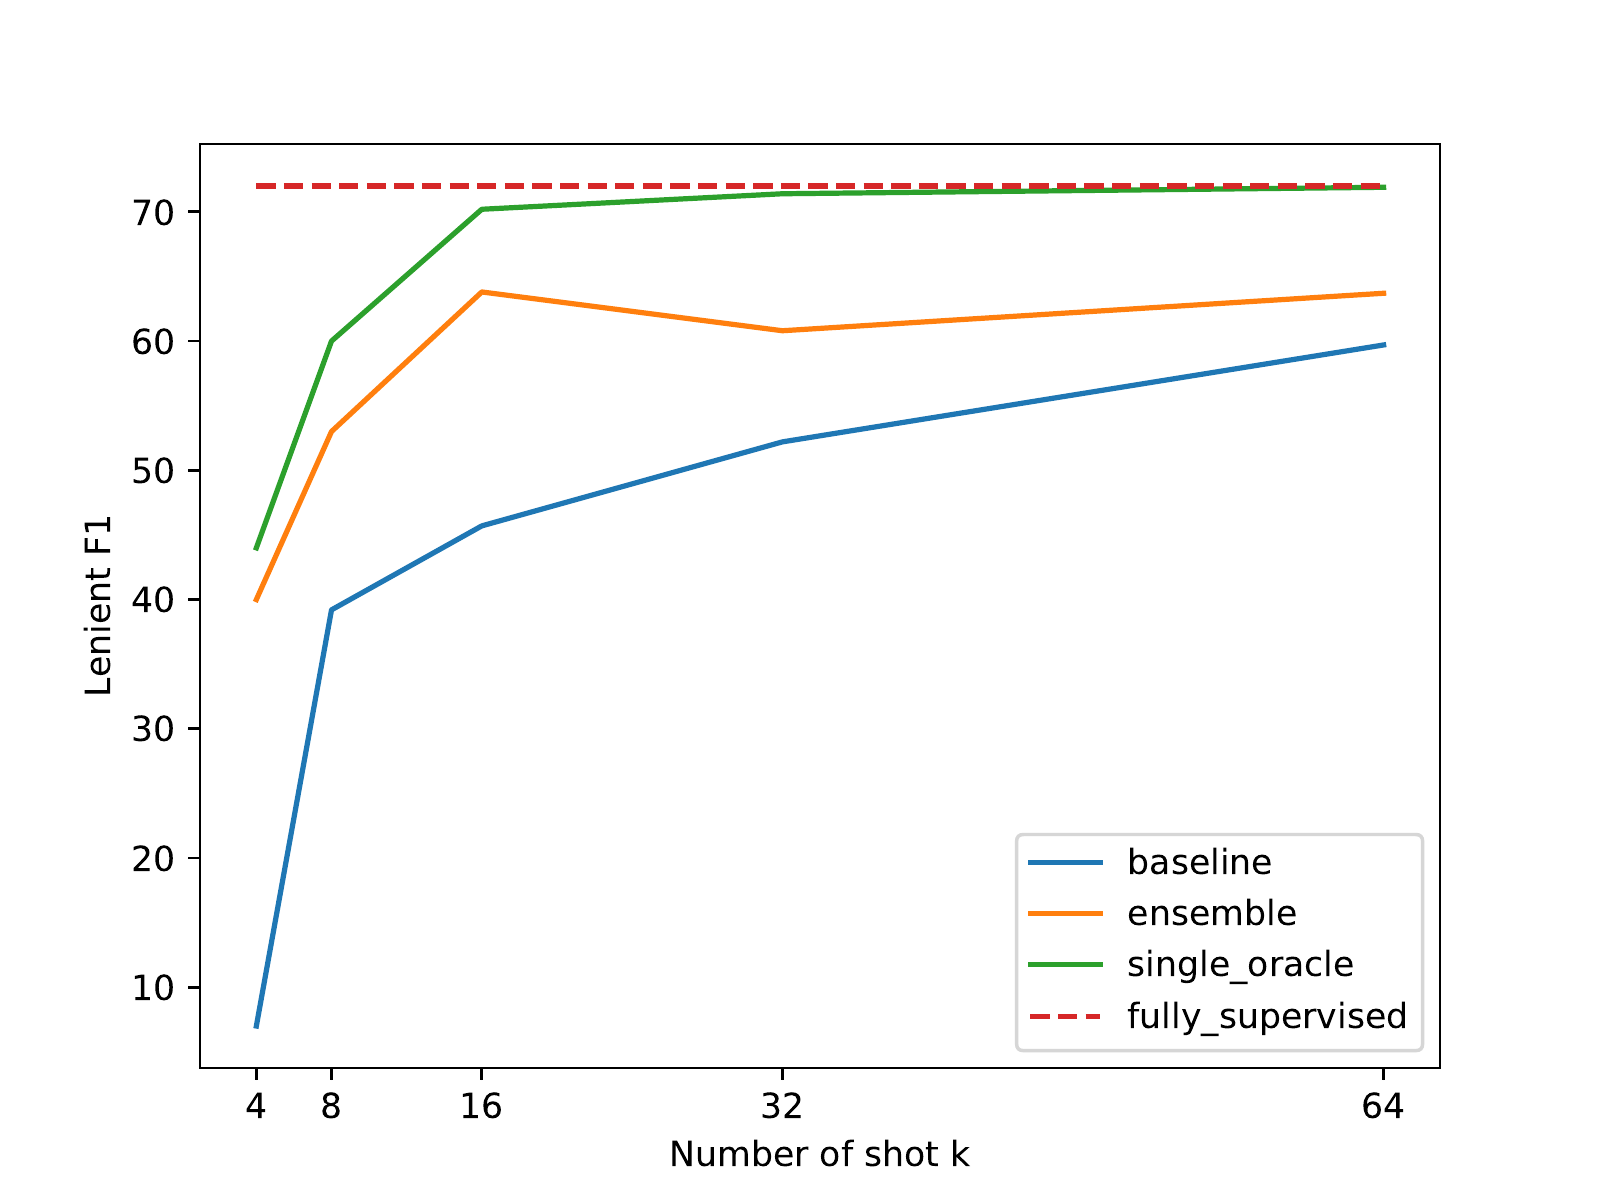}
    \caption{Results of all the in-context models as the function of number of in-context examples, for $k=16$ training set. The expectation is 2 examples would give the highest performance.}
    \label{fig:num_in_context_examples}
\end{figure}

\paragraph{Different Model Sizes} Table \ref{tab:model_sizes}
\begin{table}[!t]
\centering
\begin{tabular}{lcccc}
\hline
& \multicolumn{2}{c}{CheEMU-Ref} & \multicolumn{2}{c}{ARRAU} \\
& F1 & Acc & F1 & Acc\\
\hline
GPT-2Large & & & & \\
GPT-2XL & & & & \\
GPT-Neo & & & & \\
GPT-J & & & & \\
GPT-3 175B & & & & \\
\hline
\end{tabular}
\caption{Different foundation models, using $\mathcal{D}_{train}$ of size $k=16$}
\label{tab:model_sizes}
\end{table}

\subsection{Span-based Verbalizers Rules}
\label{app:span_based_verbalizer}
	- Current rules for ours span-based verbalizers: 
		- "x (y)" == "y of x" == "x"
		- "x, y, and z" == "x" + "y" + "z" 
		- "x in y" == "x" + "y"
	- Discussion: to make it work with annotations. Because annotations can come 
	in various forms (eg either "x in y", or, "x" and "y" separately)

\subsection{Prompt Hyperparameters}
Previous work establishes that different formats can significantly impact the in-context learning performance \cite{schick-schutze-2021-just, gao-etal-2021-making}. In this work, we mainly use QA-style format (Figure \ref{fig:approach}). We experiment with other formats and TODO conclusion (Section \ref{app:prompt_hyperparameters}). 
